# Supplementary material for: PTUM: Pre-training User Model from Unlabeled User Behaviors via Self-supervision
Source: arXiv:2010.01494 source file (2020-10-04)
Supplement: Supplementary file 1 [file supplement.tex]

\section*{Supplementary Materials}

\subsection*{Experiment Environment}
In this section, we introduce the running environments for  experiments.
All experiments are conducted on a Linux server installed with Ubuntu 16.04 operating system and Python 3.7.
The CPU type is Intel Xeon E5-2620 v4, and the type of GPU is GeForce GTX1080Ti.
The total memory is 64GB.
Each experiment is run on a single GPU and CPU core with a single process/thread.
%For word we use the NLTK tool\footnote{http://www.nltk.org/} for word tokenization.
We use the Keras\footnote{https://github.com/keras-team/} framework with tensorflow 1.12\footnote{https://github.com/tensorflow/tensorflow/releases/tag/v1.12.0} backend to implement deep learning models.

\subsection*{Dataset Construction}
In our experiments, the dataset for model pre-training and user demographic prediction are constructed by ourselves.
Both datsets are constructed via crawling the logs from a commercial platform that records user browsing behavior logs.
For the pre-training dataset, we randomly sample 500,000 users with at least one behavior (browsed webpage).
For the demographic prediction dataset, we randomly sample 20,000 users with at least one behavior and  meanwhile have both age and gender labels.
Among these users, there are 12,769 male users and 7,231 female users.
There are 103 users under twenty, 2,895 users between twenty and forty, 7,453 users between forty and sixty, and 9,549 users over sixty.

\subsection*{Preprocessing}
In our approach, the effort on preprocessing is minimal.
We first construct a dictionary of words in user behavior data, and then filter the words with low frequency ($<$30).
The rest words are converted into their IDs.
We use at most 30 words in each webpage title, and 100 behaviors of each user.
We use pre-trained Glove embeddings to initialize the word embedding matrix.

\subsection*{Hyperparameter Settings}
The hyperparameters used in our approach are summarized in Table~\ref{hyper}.

\begin{table}[h]
\centering
\resizebox{0.9\linewidth}{!}{
\begin{tabular}{|l|c|}
\hline
\multicolumn{1}{|c|}{\textbf{Hyperparameters}}& \textbf{Value} \\ \hline
word embedding dimension                     & 300            \\
\# CNN filters                               & 256          \\
LSTM hidden states dimension                  & 256         \\
\# heads in self-attention networks                 & 16             \\
output dim of self-attention head               & 16            \\
 dim of additive attention query             & 200            \\
  loss coefficient $\lambda$            & 1.0            \\
    future behavior number $K$           & 2            \\
        negative sampling ratio $P$           & 4            \\
dropout ratio                       & 0.2            \\
optimizer                                    & Adam           \\
learning rate                                & 1e-4           \\
batch size                                   & 64    \\     
Pre-training epoch                                   & 2    \\     \hline
\end{tabular}
}
\caption{Detailed settings of hyperparameters.}\label{hyper}
\end{table}

\subsection*{Model Computational Cost}

In this section, we report the computational cost of our pre-trained user model.
There are 47,626,970 parameters in PTUM, where the word embedding layer contains 47,052,900 parameters and the models contain 574,070 parameters.
The average running time of each pre-training epoch is 5,052 secs.

\subsection*{Validation Performance}
We also report the performance of different methods on the validation set.
The results are summarized in Tables~\ref{table.resultv}, \ref{table.result2v}, and \ref{table.result3v}.

\begin{table}[!t]
	\centering

	\resizebox{0.48\textwidth}{!}{
\begin{tabular}{lcccccc}
\Xhline{1.5pt}
\multirow{2}{*}{\textbf{Methods}} & \multicolumn{2}{c}{20\%}        & \multicolumn{2}{c}{50\%}        & \multicolumn{2}{c}{100\%}       \\ \cline{2-7} 
                                  & Acc.           & Macro-F        & Acc.           & Macro-F        & Acc.           & Macro-F        \\ \hline
HAN                & 51.95          & 28.59          & 53.54          & 29.68          & 55.36          & 30.99          \\
HAN+PTUM (no finetune)  & 52.35          & 28.95          & 53.75          & 29.99          & 55.42          & 31.14          \\
HAN+PTUM (finetune)         & 53.75          & 29.99          & 55.22          & 31.05          & 56.83          & 32.20          \\ \hline
HURA               & 52.09          & 28.60          & 53.86          & 29.94          & 55.64          & 31.33          \\
HURA+PTUM (no finetune) & 52.69          & 29.07          & 54.39          & 30.18          & 55.90          & 31.44          \\
HURA+PTUM (finetune)        & 54.10          & 30.15          & 55.62          & 31.49          & 57.29          & 32.59          \\ \hline
HSA                & 52.37          & 29.08          & 54.23          & 30.37          & 56.60          & 31.93          \\
HSA+PTUM (no finetune)  & 53.06          & 29.63          & 54.75          & 30.76          & 56.70          & 32.13          \\
HSA+PTUM (finetune)         & \textbf{54.59} & \textbf{30.59} & \textbf{56.18} & \textbf{31.90} & \textbf{58.09} & \textbf{33.31}
\\ \Xhline{1.5pt}
\end{tabular}
}

\caption{Results of age prediction under different ratios of training data. Static means without finetuning.}\label{table.resultv}

\end{table}

\begin{table}[!t]
	\centering
	\resizebox{0.48\textwidth}{!}{
\begin{tabular}{lcccccc}
\Xhline{1.5pt}
\multirow{2}{*}{\textbf{Methods}} & \multicolumn{2}{c}{20\%}        & \multicolumn{2}{c}{50\%}        & \multicolumn{2}{c}{100\%}       \\ \cline{2-7} 
                                  & Acc.           & Macro-F        & Acc.           & Macro-F        & Acc.           & Macro-F        \\ \hline

HAN                      & 69.99                    & 66.83                       & 72.69                    & 68.91                       & 74.08                    & 70.49                       \\
HAN+PTUM (no finetune)        & 70.37                    & 67.30                       & 72.88                    & 69.12                       & 74.19                    & 70.65                       \\
HAN+PTUM (finetune)               & 72.01                    & 68.69                       & 73.93                    & 70.12                       & 74.92                    & 71.36                       \\ \hline
HURA                     & 70.24                    & 67.08                       & 72.92                    & 69.17                       & 74.32                    & 70.93                       \\
HURA+PTUM (no finetune)       & 70.76                    & 67.58                       & 73.13                    & 69.49                       & 74.47                    & 71.14                       \\
HURA+PTUM (finetune)              & 72.20                    & 69.03                       & 74.23                    & 70.49                       & 75.25                    & 71.80                       \\ \hline
HSA                      & 70.46                    & 67.34                       & 73.25                    & 69.42                       & 74.91                    & 71.57                       \\
HSA+PTUM (no finetune)        & 71.00                    & 67.79                       & 73.51                    & 69.74                       & 75.12                    & 71.78                       \\
HSA+PTUM (finetune)               & 72.52                    & 69.26                       & 74.61                    & 70.78                       & 75.88                    & 72.48 \\                     
\Xhline{1.5pt}
\end{tabular}
}

\caption{Results of gender prediction under different ratios of training data. Static means without finetuning.}\label{table.result2v}

\end{table}

\begin{table}[!t]
	\centering
\resizebox{0.48\textwidth}{!}{
\begin{tabular}{lcccccc}
\Xhline{1.5pt}
\multirow{2}{*}{\textbf{Methods}} & \multicolumn{2}{c}{20\%}        & \multicolumn{2}{c}{50\%}        & \multicolumn{2}{c}{100\%}       \\ \cline{2-7} 
                                  & AUC            & AP             & AUC            & AP             & AUC            & AP             \\ \hline
GRU4Rec                & 71.49          & 73.35          & 72.01          & 74.02          & 72.34          & 74.58          \\
GRU4Rec+PTUM (no finetune)  & 71.96          & 73.88          & 72.15          & 74.33          & 72.53          & 74.99          \\
GRU4Rec+PTUM (finetune)         & 72.55          & 74.71          & 72.63          & 74.94          & 72.95          & 75.56          \\ \hline
AttCTR                 & 71.83          & 73.63          & 72.11          & 74.16          & 72.57          & 74.74          \\
AttCTR+PTUM (no finetune)   & 72.19          & 74.10          & 72.32          & 74.51          & 72.66          & 75.14          \\
AttCTR+PTUM (finetune)          & 72.74          & 75.00          & 72.75          & 75.10          & 73.14          & 75.71          \\ \hline
BERT4Rec               & 71.99          & 74.15          & 72.55          & 75.02          & 73.13          & 75.66          \\
BERT4Rec+PTUM (no finetune) & 72.32          & 74.69          & 72.75          & 75.36          & 73.34          & 75.97          \\
BERT4Rec+PTUM (finetune)        & \textbf{72.91} & \textbf{75.56} & \textbf{73.23} & \textbf{76.04} & \textbf{73.73} & \textbf{76.62} \\
\Xhline{1.5pt}
\end{tabular}
}

\caption{Results of ad CTR prediction on the validation set under different ratios of training data. }\label{table.result3v}
	
\end{table}

\begin{figure}[t]
	\centering
\subfigure[\textit{Demo} Dataset.]{\label{fig.la}
	\includegraphics[width=0.22\textwidth]{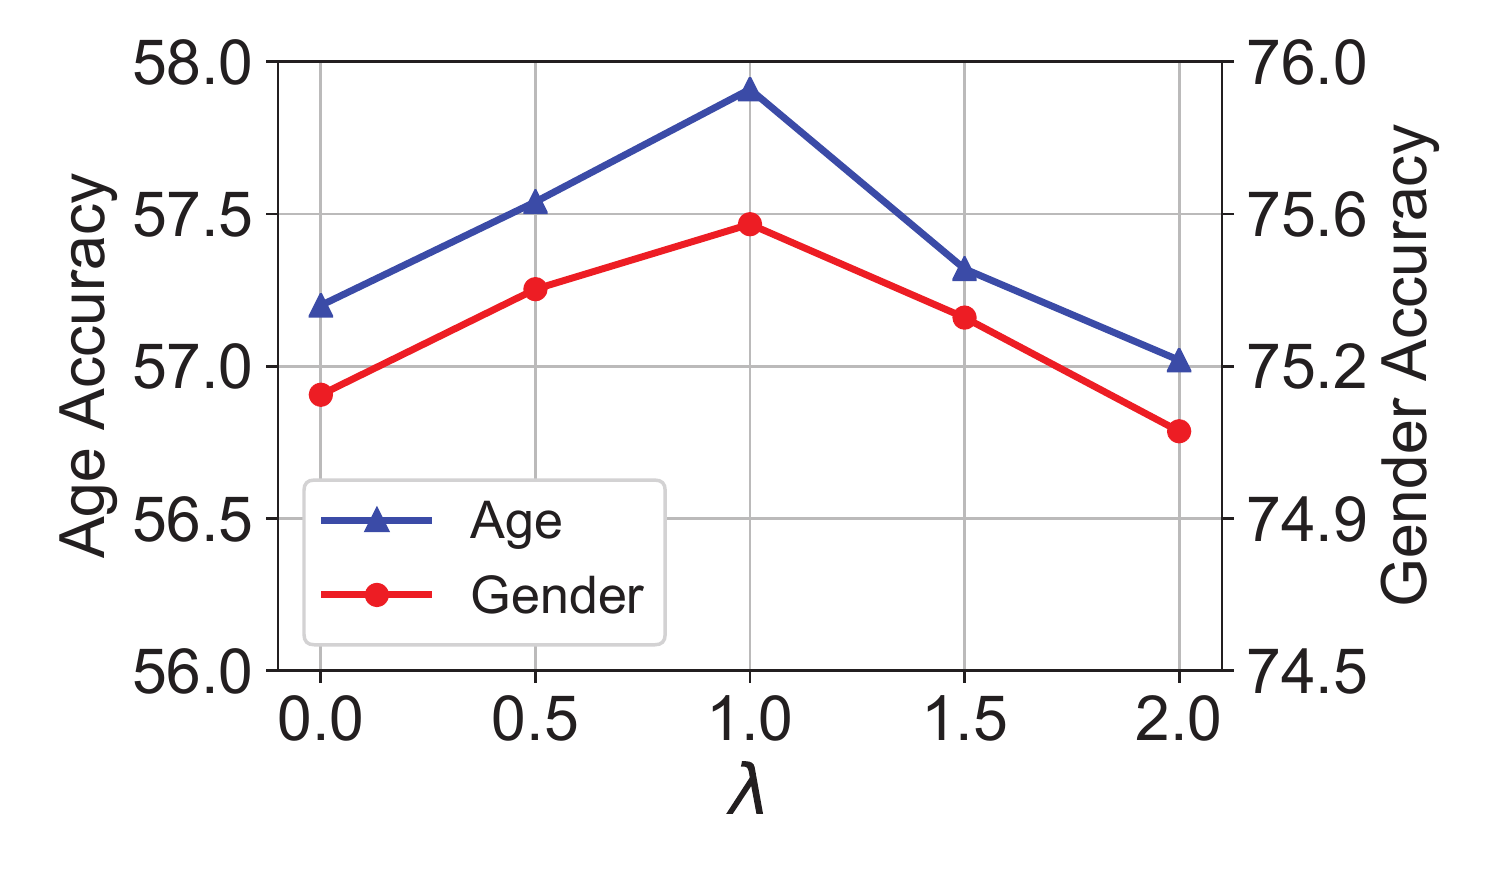}   
	}
	\subfigure[\textit{CTR} Dataset.]{\label{fig.lb}
	\includegraphics[width=0.22\textwidth]{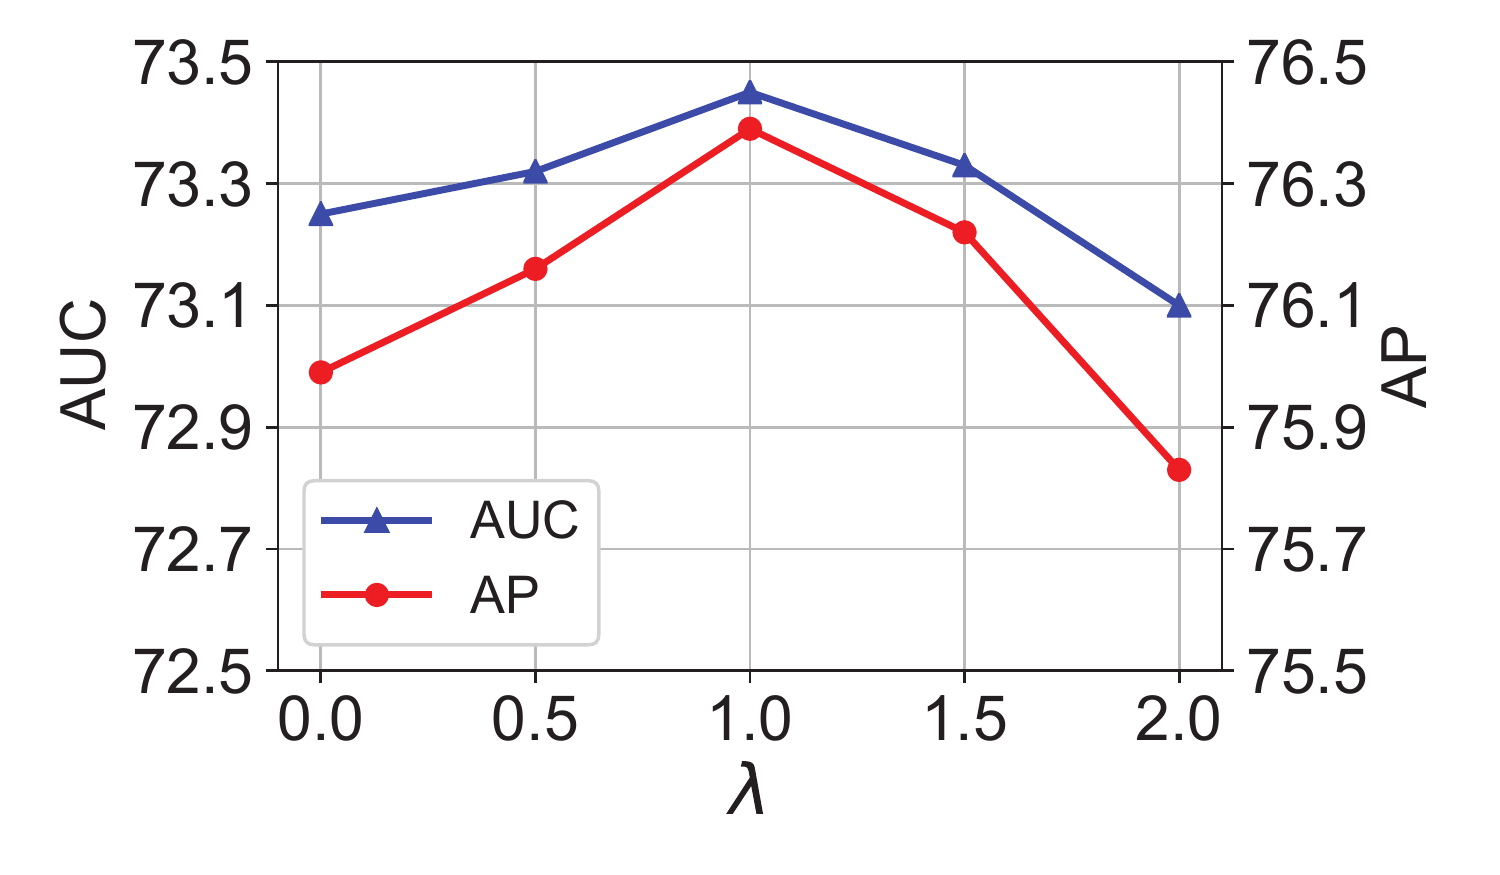}   
	}  % \vspace{-0.05in}
\caption{Performance of \textit{PTUM} w.r.t. different $\lambda$. }    %\vspace{-0.05in}
\end{figure}

\subsection*{Hyper-parameter Analysis}
In this section, we explore the influence of two key hyper-parameters on our approach, i.e., the coefficient $\lambda$ in Eq. (\ref{loss}) and the number of behavior $K$ in the NBP task.
We first vary the coefficient $\lambda$ to compare the performance of pre-trained \textit{HSA} w.r.t. different $\lambda$, and the results on the \textit{Demo} and \textit{CTR} datasets are shown in Figs.~\ref{fig.la} and~\ref{fig.lb}.
From these results, we find the performance is not optimal under a small $\lambda$.
This may be because the useful self-supervision signals in the NBP task is not fully exploited.
When $\lambda$ goes too large, the performance begins to decline.
This may be because the NBP task is over-emphasized and the MBP task is not well pre-trained.
Thus, it may be more suitable to set $\lambda=1$ to balance the two tasks.

Then, we vary the behavior number $K$ to explore its influence on the performance of \textit{PTUM}, and the results are shown in Figs.~\ref{fig.hypera} and~\ref{fig.hyperb}.
According to these results, we find that the performance of pre-trained user models in downstream tasks is not optimal at $K=1$.
This is probably because the relatedness between the last input behavior and the first behavior in the future may be strong, and the model may tend to overfit their short-term relatedness.
Thus, it is not optimal to simply predict the next one behavior.
In addition, we find the performance is sub-optimal when $K$ is too large.
This may be because it is difficult to accurately predict user behaviors in a long term due to the diversity of user behaviors.
Thus, a moderate $K$ may be more appropriate (e.g., $K=2$).

\begin{figure}[t]
	\centering
\subfigure[\textit{Demo} Dataset.]{\label{fig.hypera}
	\includegraphics[width=0.22\textwidth]{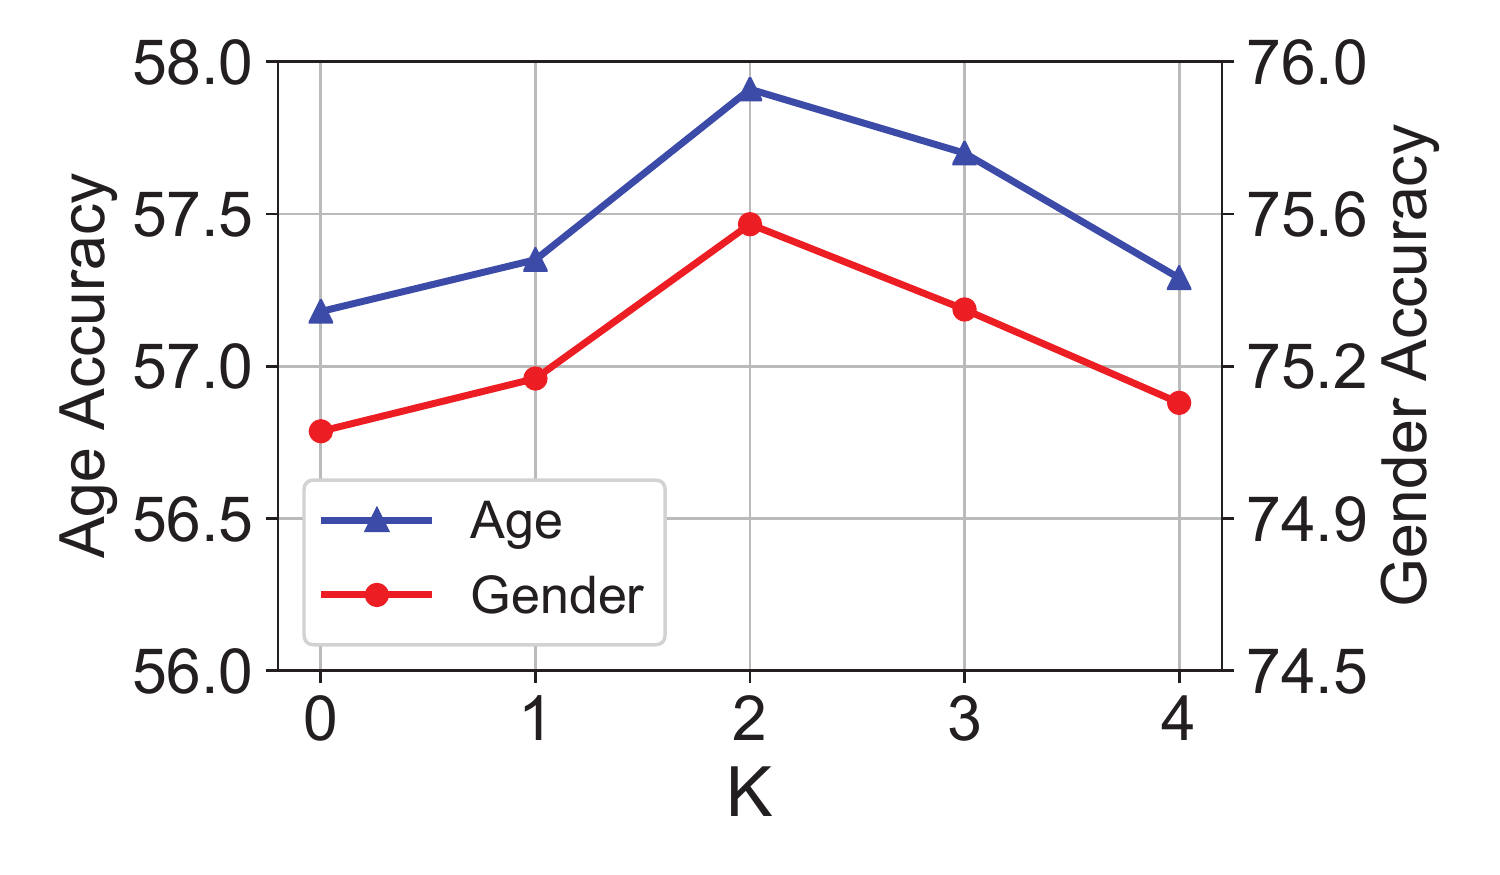}  
	}
	\subfigure[\textit{CTR} Dataset.]{\label{fig.hyperb}
	\includegraphics[width=0.22\textwidth]{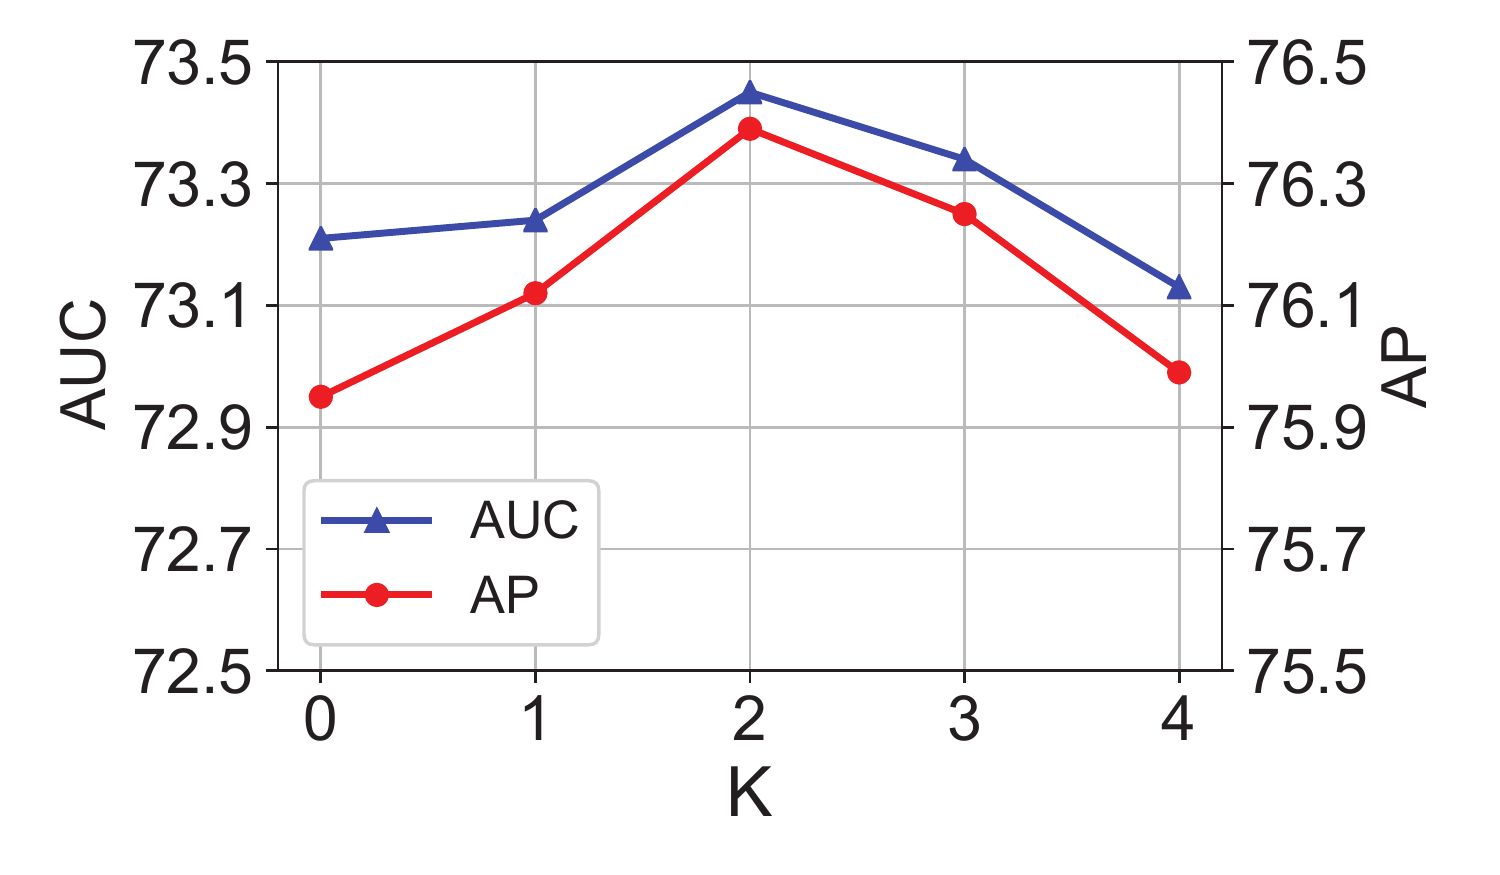}
	}  % \vspace{-0.05in}
\caption{Performance of \textit{PTUM} w.r.t. different $K$. }    %\vspace{-0.05in}
\end{figure}
